# Supplementary material for: Generalised Einstein Relation for Hot Brownian Motion
Source: arXiv:1110.3734 ancillary file (2011-10-18)
Supplement: Supplementary file 1 [file supmat.pdf]

# Generalised Einstein Relation for Hot Brownian Motion: Supporting Information

D. Chakraborty, M. V. Gnann, D. Rings, J. Glaser, F. Otto, F. Cichos, and K. Kroy

**Abstract**

Here we provide some technical and supplementary information: a detailed formulation of the contraction of the fluctuating hydrodynamics problem to a Markovian Langevin description of the Brownian motion of the nanoparticle, convenient analytical approximations for $T_{\mathrm{HBM}}$ and $D_{\mathrm{HBM}}$, a discussion of how to deal with finite size effects in the numerical simulations, information about the parallel processing of the simulation code, and various supporting plots.

## 1 Fluctuating hydrodynamics

The previous derivation of $T_{\mathrm{HBM}}$ by Rings *et al.* [4, 5] employed a thermodynamic argument that yields exact results under isothermal conditions but amounts to an approximation in the non-equilibrium case. It is correct to first order in the temperature difference $\Delta T$ between the ambient temperature $T_0$ and the solvent temperature at the surface of the particle [4, 5]. To this order, the temperature dependence of the viscosity and the thermal conductivity do not enter. But, in order to obtain the correct $T_{\mathrm{HBM}}$ in higher orders, it is crucial to properly include the fluctuations of the solvent velocity. According to eq. (3) of the main text, they render $T_{\mathrm{HBM}}$ larger than found from the thermodynamic argument that neglects fluctuations, corresponding to a weighted average of $1/T$ instead of $T$. The superiority of the resulting approximation for aqueous suspensions, eq. (5) of the main text, and, in general, of the exact prediction, presented below, over the previous (thermodynamic) estimates of $T_{\mathrm{HBM}}$ becomes noticeable at temperature increments $\Delta T \simeq T_0$. These are conveniently studied in our numerical simulations.

**Derivation** As pointed out in Ref. [5], our starting point is a fluctuating hydrodynamics description. We therefore split the fluid velocity and the pressure into a systematic part $(\mathbf{u}, p)$ and a random part $(\tilde{\mathbf{u}}, \tilde{p})$ that obey

$$\nabla \cdot \sigma(\mathbf{r}, t) = 0, \quad t \geq 0, \, \mathbf{r} \in V, \tag{1a}$$

$$\nabla \cdot \mathbf{u}(\mathbf{r}, t) = 0, \quad t \geq 0, \, \mathbf{r} \in V, \tag{1b}$$

$$\mathbf{u}(\mathbf{r}, t) = \mathbf{U}(t) + \mathbf{\Omega}(t) \times \mathbf{r}, \quad t \geq 0, \, \mathbf{r} \in \partial B \tag{1c}$$

and

$$\nabla \cdot \tilde{\sigma}(\mathbf{r},t) = -\nabla \cdot \tilde{\tau}(\mathbf{r},t), \;\; t \geq 0, \, \mathbf{r} \in V, \tag{2a}$$

$$\nabla \cdot \tilde{\mathbf{u}}(\mathbf{r},t) = 0, \;\; t \geq 0, \, \mathbf{r} \in V, \tag{2b}$$

$$\tilde{\mathbf{u}}(\mathbf{r},t) = 0, \;\; t \geq 0, \, \mathbf{r} \in \partial B, \tag{2c}$$

where $\sigma_{ij} = 2\eta\Gamma_{ij} - \delta_{ij}p$ ($\tilde{\sigma}_{ij} = 2\eta\tilde{\Gamma}_{ij} - \delta_{ij}\tilde{p}$), with $\mathsf{\Gamma} = (\nabla\mathbf{u} + \nabla\mathbf{u}^T)/2$ ($\tilde{\mathsf{\Gamma}} = (\nabla\tilde{\mathbf{u}}+\nabla\tilde{\mathbf{u}}^T)/2$), denotes the systematic (random) stress tensor and $(\mathbf{U}(t), \mathbf{\Omega}(t))$ the velocity and angular momentum of the Brownian particle $B$. The sum $(\mathbf{u}+\tilde{\mathbf{u}}, p+\tilde{p})$ then obeys the inhomogeneous Stokes problem with inhomogeneous boundary conditions. Note that $B$ denotes the interior of the Brownian particle, while $\bar{B}$ and $\partial B$ denote its closure and boundary. Then, the volume $V$ is given by $V = \mathbb{R}^3 \setminus \bar{B}$. (The following argumentation can be easily generalised to bounded volumes $V$ by choosing appropriate boundary conditions on $\partial V \setminus \partial B$ for the fluid velocity). The motion of the Brownian particle is described by Newton's law, viz.

$$m\dot{\mathbf{U}}(t) = -\int_{\partial B} (\sigma(\mathbf{r},t) + \tilde{\sigma}(\mathbf{r},t)) \cdot \mathbf{n}(\mathbf{r}) \, \mathrm{d}^2 r \,, \tag{3a}$$

$$\mathsf{J} \cdot \dot{\mathbf{\Omega}}(t) = -\int_{\partial B} \mathbf{r} \times [(\sigma(\mathbf{r},t) + \tilde{\sigma}(\mathbf{r},t)) \cdot \mathbf{n}(\mathbf{r})] \, \mathrm{d}^2 r \,. \tag{3b}$$

Here $\mathbf{n}(\mathbf{r})$ denotes the inner normal field of $B$ and $m$ and $\mathsf{J}$ the mass of the Brownian particle and the tensor of inertia. Eqs. (1), (2), and (3) are complemented by

$$\langle \tilde{\tau}_{ij}(\mathbf{r},t)\tilde{\tau}_{kl}(\mathbf{r}',t') \rangle \;=\; 2\eta(\mathbf{r},t)k_{\mathrm{B}}T(\mathbf{r},t)\delta(\mathbf{r}-\mathbf{r}')\delta(t-t')\left[\delta_{ik}\delta_{jl} + \delta_{il}\delta_{jk}\right] \;, \tag{4}$$

(and $\tilde{\tau} = 0$ on $\partial B$) which specifies the two-point correlations for the Gaussian white noise representing the thermal stress fluctuations in the fluid according to the local equilibrium assumption. For a discussion of choosing proper boundary conditions for $\tilde{\tau}$ we refer to Ref. [2].

Our aim is to achieve a contraction of the problem by integrating out the fluid variables following Ref. [2]. We therefore define

$$\mathbf{b}(t) = \begin{pmatrix} \mathbf{U}(t) \\ \mathbf{\Omega}(t) \end{pmatrix}, \;\; \mathsf{L} := \begin{pmatrix} m & 0 \\ 0 & \mathsf{J} \end{pmatrix},$$

obeying a linear Langevin equation of the form

$$\mathsf{L} \cdot \dot{\mathbf{b}}(t) = \mathbf{h}(t) + \tilde{\mathbf{h}}(t), \tag{5}$$

where

$$\mathbf{h}(t) = -\int_{\partial B} \begin{pmatrix} \sigma(\mathbf{r},t) \cdot \mathbf{n}(\mathbf{r}) \\ \mathbf{r} \times [\sigma(\mathbf{r},t) \cdot \mathbf{n}(\mathbf{r})] \end{pmatrix} \mathrm{d}^2 r \,, \tag{6a}$$

$$\tilde{\mathbf{h}}(t) = -\int_{\partial B} \begin{pmatrix} \tilde{\sigma}(\mathbf{r},t) \cdot \mathbf{n}(\mathbf{r}) \\ \mathbf{r} \times [\tilde{\sigma}(\mathbf{r},t) \cdot \mathbf{n}(\mathbf{r})] \end{pmatrix} \mathrm{d}^2 r \tag{6b}$$

are systematic and random forces and torques acting on $B$.

Since eq. (1) is linear, velocity and pressure fields $\mathbf{u}(\mathbf{r},t)$ and $p(\mathbf{r},t)$ are linear functionals of $\mathbf{b}(t)$ subject to the boundary conditions (1c). Moreover, since by eq. (6a) $\mathbf{h}(t)$ is a linear functional of $\mathbf{b}(t)$, we can write

$$\mathbf{h}(t) = -\mathsf{Z}\cdot\mathbf{b}(t). \tag{7}$$

The positive semidefinite friction tensor $\mathsf{Z}$ is defined by specifying its quadratic form $\mathbf{b}\cdot\mathsf{Z}\cdot\mathbf{b}$ for arbitrary, but time-independent, $\mathbf{b}$. Using antisymmetry of the box product under transpositions and Gauss' integral theorem, we gain

$$\begin{aligned}
\mathbf{b}\cdot\mathsf{Z}\cdot\mathbf{b} &= \int_{\partial B}\mathbf{U}\cdot\sigma(\mathbf{r},t)\cdot\mathbf{n}(\mathbf{r})\,\mathrm{d}^2r + \int_{\partial B}\mathbf{\Omega}\cdot[\mathbf{r}\times(\sigma(\mathbf{r},t)\cdot\mathbf{n}(\mathbf{r}))]\,\mathrm{d}^2r \\
&= \int_{\partial B}[\mathbf{U}+\mathbf{\Omega}\times\mathbf{r}]\cdot[\sigma(\mathbf{r},t)\cdot\mathbf{n}(\mathbf{r})]\,\mathrm{d}^2r \\
&\overset{(1c)}{=} \int_{\partial B}[(\mathbf{u}(\mathbf{r},t))\cdot\sigma(\mathbf{r},t)]\cdot\mathbf{n}(\mathbf{r})\,\mathrm{d}^2r \\
&= \int_V \nabla\cdot[\sigma(\mathbf{r},t)\cdot\mathbf{u}(\mathbf{r},t)]\,\mathrm{d}^3r \\
&= \int_V [(\partial_i\sigma_{ij})u_j + \sigma_{ij}\partial_i u_j]\,\mathrm{d}^3r \\
&\overset{(1a)}{=} \int_V \sigma_{ij}\partial_i u_j\,\mathrm{d}^3r \\
&= \int_V [\eta(\partial_i u_j + \partial_j u_i) - p\delta_{ij}]\,\partial_i u_j\,\mathrm{d}^3r \\
&\overset{(1b)}{=} \int_V \phi(\mathbf{r},t)\,\mathrm{d}^3r,
\end{aligned} \tag{8}$$

where we used the definition of the dissipation function $\phi(\mathbf{r},t)$ as

$$\phi = \eta\,[(\partial_i u_j)(\partial_i u_j) + (\partial_i u_j)(\partial_j u_i)]\ .$$

Due to the structure of eq. (2) and the representation of the random forces by eq. (6b), $\tilde{\mathbf{h}}(t)$ describes Gaussian white noise, too. It therefore suffices to characterise the two-point correlation matrix $\langle\tilde{\mathbf{h}}(t)\otimes\tilde{\mathbf{h}}(t')\rangle$, which is positive semidefinite. Hence, we fix an arbitrary $\mathbf{b}\in\mathbb{R}^6$ and calculate the correlations

$$\mathbf{b}\cdot\langle\tilde{\mathbf{h}}(t)\otimes\tilde{\mathbf{h}}(t')\rangle\cdot\mathbf{b} = \langle(\mathbf{b}\cdot\tilde{\mathbf{h}}(t))\,(\mathbf{b}\cdot\tilde{\mathbf{h}}(t'))\rangle\,.$$

Then, we find

$$
\begin{aligned}
\mathbf{b}\cdot\tilde{\mathbf{h}}(t) &= -\mathbf{U}\cdot\int_{\partial B}\tilde{\sigma}(\mathbf{r},t)\cdot\mathbf{n}(\mathbf{r})\,\mathrm{d}^2r-\boldsymbol{\Omega}\int_{\partial B}\mathbf{r}\times[\tilde{\sigma}(\mathbf{r},t)\cdot\mathbf{n}(\mathbf{r})]\,\mathrm{d}^2r\\
&= \int_{\partial B}[\mathbf{U}+\boldsymbol{\Omega}\times\mathbf{r}]\cdot[\tilde{\sigma}(\mathbf{r},t)\cdot\mathbf{n}(\mathbf{r})]\,\mathrm{d}^2r\\
&\overset{(1c)}{=} \int_{\partial B}[(\mathbf{u}(\mathbf{r},t))\cdot\tilde{\sigma}(\mathbf{r},t)]\cdot\mathbf{n}(\mathbf{r})\,\mathrm{d}^2r\\
&= \int_V\nabla\cdot[\tilde{\sigma}(\mathbf{r},t)\cdot\mathbf{u}(\mathbf{r},t)]\,\mathrm{d}^3r\\
&= \int_V[(\partial_i\tilde{\sigma}_{ij})u_j+\tilde{\sigma}_{ij}\partial_iu_j]\,\mathrm{d}^3r\\
&\overset{(2a)}{=} -\int_V(\partial_i\tilde{\tau}_{ij})u_j\,\mathrm{d}^3r+\int_V[\eta(\partial_i\tilde{u}_j+\partial_j\tilde{u}_i)-\tilde{p}\delta_{ij}]\,\partial_iu_j\,\mathrm{d}^3r\\
&\overset{(1b)}{=} -\int_V(\partial_i\tilde{\tau}_{ij})u_j\,\mathrm{d}^3r+\int_V\frac{\eta}{2}(\partial_i\tilde{u}_j+\partial_j\tilde{u}_i)(\partial_iu_j+\partial_ju_i)\,\mathrm{d}^3r\\
&\overset{(2b)}{=} -\int_V(\partial_i\tilde{\tau}_{ij})u_j\mathrm{d}^3r+\int_V\sigma_{ij}\partial_i\tilde{u}_j\,\mathrm{d}^3r\\
&\overset{(2c)}{=} -\int_V(\partial_i\tilde{\tau}_{ij})u_j\mathrm{d}^3r-\int_V(\partial_i\sigma_{ij})\,\tilde{u}_j\,\mathrm{d}^3r\\
&\overset{(1a)}{=} \int_V\tilde{\tau}_{ij}\partial_iu_j\,\mathrm{d}^3r\;.
\end{aligned}
$$

In the last equality we also used the property $\tilde{\tau}=0$ on $\partial B$. Using this result for the two-point correlations of $\tilde{\mathbf{h}}$, we gain

$$
\begin{aligned}
&\mathbf{b}\cdot\left\langle\tilde{\mathbf{h}}(t)\otimes\tilde{\mathbf{h}}(t')\right\rangle\cdot\mathbf{b}\\
&= \int_V\int_V(\partial_iu_j(\mathbf{r},t))(\partial_ku_l(\mathbf{r}',t'))\left\langle\tilde{\tau}_{ij}(\mathbf{r},t)\tilde{\tau}_{kl}(\mathbf{r}',t')\right\rangle\mathrm{d}^3r\,\mathrm{d}^3r'\\
&\overset{(4)}{=} \int_V 2\eta(\mathbf{r},t)k_\mathrm{B}T(\mathbf{r},t)\delta(t-t')\\
&\quad\times[(\partial_iu_j(\mathbf{r},t))(\partial_iu_j(\mathbf{r},t'))+(\partial_iu_j(\mathbf{r},t))(\partial_ju_i(\mathbf{r},t'))]\,\mathrm{d}^3r\\
&= \int_V 2k_\mathrm{B}T(\mathbf{r},t)\delta(t-t')\phi(\mathbf{r},t)\,\mathrm{d}^3r\;.
\end{aligned}
\tag{9}
$$

Comparison with eq. (8) yields

$$
\left\langle\tilde{\mathbf{h}}(t)\otimes\tilde{\mathbf{h}}(t')\right\rangle=2\mathsf{Z}k_\mathrm{B}T_\mathrm{HBM}\delta(t-t'),\tag{10}
$$

with $T_\mathrm{HBM}$ given by

$$
T_\mathrm{HBM}=\frac{\int_V T(\mathbf{r},t)\phi(\mathbf{r},t)\,\mathrm{d}^3r}{\int_V\phi(\mathbf{r},t)\,\mathrm{d}^3r}\;,\tag{11}
$$

its time-independent version being stated in eq. (3) of the main text.

# 2 Approximate formulas for $D_\mathrm{HBM}$ and $T_\mathrm{HBM}$

The above eq. (11), corresponding to eq. (3) of the main text, provides a new, exact expression for the effective temperature $T_\mathrm{HBM}$. In eq. (6) of the main text, we evaluate this expression approximately to obtain the analytical formula

$$
T_\mathrm{HBM}\approx T_0+\frac{5}{12}\Delta T+\frac{\ln(\eta_0/\eta_\infty)}{22(T_0+\Delta T-T_\mathrm{VF})}\,\Delta T^2\tag{12}
$$

for practical applications, which supersedes previous estimates [4, 5] based on a thermodynamic approximation to eq. (3) of the main text. The general structure of the second order term (with the surface temperature $T_0 + \Delta T$ appearing in the denominator) is that of a Padé approximation of the higher order corrections to the exact first order result, calculated with the analytical toy model introduced in Refs. [4, 5]. The numerical factor 22 has been chosen by hand to improve the fit to exact numerical results obtained from the shell method calculation for water.

The previous prediction for the effective friction $\zeta_{\rm HBM}$ [4, 5] is not affected by our new results. Thus, for a temperature dependence of the solvent viscosity of the form $\eta(T) = \eta_\infty \exp[A/(T - T_{\rm VF})]$, the analytic approximation for $\zeta_{\rm HBM}$ given in eq. (75) of Ref. [5],

$$\frac{\eta_0}{\eta_{\rm HBM}} \approx 1 + \frac{193}{486}\left[\ln\frac{\eta_0}{\eta_\infty}\right]\theta - \left[\frac{56}{243}\ln\frac{\eta_0}{\eta_\infty} - \frac{12563}{118098}\ln^2\frac{\eta_0}{\eta_\infty}\right]\theta^2 \,, \tag{13}$$

with $\theta \equiv \Delta T/(T_0 - T_{\rm VF})$, remains an excellent estimate. However, the diffusion coefficient $D_{\rm HBM}$, which is obtained as the ratio of $T_{\rm HBM}$ and $\zeta_{\rm HBM}$ via the generalised Einstein relation, eq. (1) of the main text, has to be reevaluated. We found that a good approximation for $D_{\rm HBM}$ is obtained by combining eq. (13) with the second order Taylor series expansions of the analytic toy-model approximation for $T_{\rm HBM}$,

$$T_0 + \frac{\Delta T}{2} + \frac{A\Delta T^2}{12(T_0 - T_{\rm VF})^2} \,, \tag{14}$$

rather than with eq. (12). Excellent agreement (to within 3% for $\Delta T < T_0$) with the exact numerical result from the differential shell method [5] is achieved by multiplying the second order term of the product of (14) and (13) by a factor 2/3 in an attempt to incorporate higher order corrections. This yields the semi-empirical formula

$$\begin{aligned} D_{\rm HBM}\cdot\frac{6\pi\eta_0 R}{k_{\rm B}T_0} \approx 1 &+ \left(\frac{193}{486}\ln\frac{\eta_0}{\eta_\infty} + \frac{1}{2}\Big(1 - \frac{T_{\rm VF}}{T_0}\Big)\right)\theta \\ &- \frac{2}{3}\left(\left[\frac{56}{243} - \frac{137}{486}\Big(1 - \frac{T_{\rm VF}}{T_0}\Big)\right]\ln\frac{\eta_0}{\eta_\infty} - \frac{12563}{118098}\left[\ln\frac{\eta_0}{\eta_\infty}\right]^2\right)\theta^2 \,, \end{aligned} \tag{15}$$

which may serve as a replacement for eq. (82) of Ref. [5].

For the Lennard-Jones system, an accurate approximation for $T_{\rm HBM}$, different from eq. (12), can be obtained along similar lines. Due to the different temperature-dependence of the Lennard-Jones viscosity, namely

$$\ln\left[\eta(T)/\eta_\infty\right] = (A/T)^4 \,, \tag{16}$$

as given in eq. (9) of the main text, the second order Padé-type approximation obtained in the same way as eq. (12),

$$T_0 + \frac{\Delta T}{2} - \frac{\Delta T^2\left(-4A^4 + T_0^4\right)^2}{6\Delta T T_0^4\left(-20A^4 + T_0^4\right) + 12T_0^4\left(-4A^4 T_0 + T_0^5\right)} \,, \tag{17}$$

needs a more subtle adaptation to turn it into a numerically precise semi-empirical formula of comparable quality as eq. (12). By multiplying the first

summand in the denominator of the last term by 6, we get

$$T_{\text{HBM}} \approx T_0 + \frac{\Delta T}{2} - \frac{1 - 4\ln(\eta_0/\eta_\infty)}{12\,(T_0 + 3\Delta T[1 - 20\ln(\eta_0/\eta_\infty)]/[1 - 4\ln(\eta_0/\eta_\infty)])}\Delta T^2\,, \tag{18}$$

which fits the exact numerical result to within 3% for $\Delta T \leq T_0$.

# 3 Implementation details of the MD simulation

In the following lines, we briefly describe the details of our implementation of the molecular dynamics simulations. The large scale MD simulations were implemented on graphics processing units (GPUs). We chose the atom decomposition method for our parallel implementation, in which a single thread was assigned the task of updating the coordinates and momenta of a particle. A GPU-optimised cell list algorithm was used to construct the Verlet list for the system. The first step in the construction of the Verlet list was the sorting of particles into their respective cells. The system was divided into cubes with sides of length $r_c + r_s$, where $r_c$ is the potential cutoff of $2.5\sigma$ and $r_s$ is the skin length [1]. The particles were assigned three integers $n_i \equiv \lfloor x_i/L \rfloor$, which identify to which cell each particle belongs. Using a parallel radixsort algorithm, the particles were then sorted into their respective cells. The particle indices contained in the 26 neighboring cells of a given cell were loaded into the shared memory. However, the limited size of the shared memory prevented a simultaneous copying of the particle coordinates. Instead, the particle coordinates were loaded from the textures and an iterative search was then made for the neighbor lookup.

The Nosé-Hoover equations of motion [3] were integrated using the implicit Leap-Frog integration scheme [6]. The numerical stability of the scheme was monitored by recording the total energy and total momentum of the system. During the heating of the nanoparticle, the global Nosé-Hoover thermostat was switched off, and the temperature both of the colloid and of the solvent near the container boundaries were controlled by velocity rescaling.

# 4 Finite size effects

To estimate the finite size effects in the simulations of a free Brownian nanoparticle, measurements of the effective diffusion and friction coefficients $D_{\text{HBM}}$ and $\zeta_{\text{HBM}}$ were performed for different side lengths $L$ of the simulation box. Care was taken to adjust the solvent temperature at the boundary, such that the measured $T(r)$ was identical to that obtained for the largest simulation box, as demonstrated in the left panel of figure 1. A similar approach was taken for the measurement of $T_{\text{HBM}}$ for a harmonically confined hot Brownian particle. In the right panel, we show the variation of the effective temperature $T_{\text{HBM}}$ for different values of the dimensionless ratio $R/L$, with $R$ being the nanoparticle's radius.

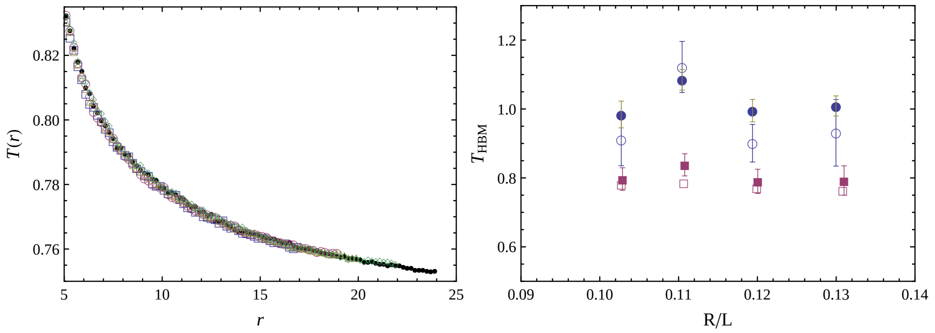


Figure 1: **Left**: Radial temperature profile around the nanoparticle kept at an elevated temperature of $T_\mathrm{p} = 1$ for five different sizes of the simulation box, $L = 37.22$ (□); $L = 40.62$ (○); $L = 44.01$ (△); $L = 47.40$ (◇) and $L = 50.78$ ( •). **Right**: Dependence of the effective temperature $T_\mathrm{HBM}$ on the dimensionless number $R/L$ for two temperatures of the nanoparticle, $T_\mathrm{p} = 1.00$ ( ●,○) and $T_\mathrm{p} = 2.25$ (■,□). The open and filled symbols are for a free and confined hot Brownian particle, respectively.

# 5 Hot Brownian motion in external fields

Figure 2 compares the simulation results for a hot nanoparticle in traps of various strengths $K$ (including $K = 0$, corresponding to a free particle) to prove that the characterization of the thermal motion by the effective temperatures $T_\mathrm{HBM}$ and $T_\mathrm{k}$ holds irrespective of the presence of external harmonic (left) and anharmonic (right) potentials.

# 6 Dependence on the heating mechanism

In our nonequilibrium simulations, the temperature control was realised by rescaling the velocities of the individual atoms to be cooled or heated. We used two protocols of rescaling: with and without conserving the center-of-mass momentum of the cooled/heated group of atoms, corresponding to internal and external physical heating mechanisms, respectively. (For example, if the nanoparticle is imagined to be heated by an internal chemical reaction, one would like to conserve its center-of-mass momentum upon heating.) In both cases, the total momentum of the whole simulated system was kept equal to zero within machine precision. We measured the distribution of the configurational and kinetic degrees of freedom for two particle temperatures $T_\mathrm{p}$ in a harmonic potential of spring constant $\kappa = 1$. Within statistical error bars, the configurational temperature $T_\mathrm{HBM}$ was independent of the rescaling procedure. In contrast, the values obtained for the kinetic temperature $T_\mathrm{k}$ differed by almost 8 times the standard error in the two heating scenarios (see figure 3).

# 7 Independence of the particle solubility

The effective temperatures $T_\mathrm{HBM}$ and $T_\mathrm{k}$ were determined for various particle solubilities. We changed the wetting properties of the colloid surface

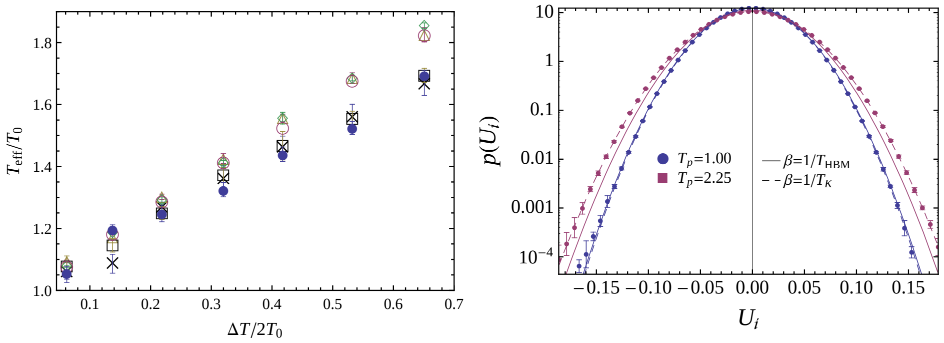


Figure 2: **Left**: Effective temperatures for the Boltzmann distribution in a harmonic trap of stiffness $K$: $T_{\rm HBM}$ for $K = 0$ •, $K = 30$ ×, $K = 50$ □ and $T_{\rm k}$ for $K = 0$ ○, $K = 30$ △, $K = 50$ ◇; filled and open circles as in Figure 3 of the main text. **Right**: The distribution of the velocities of a hot Brownian particle in the asymmetric and anharmonic potential $v(x) = Kx^4/4 + bx$ (corresponding distributions for the position coordinates are depicted in the lower panel of Figure 4 of the main text).

by modifying the range of attraction in the Lennard-Jones potential $U(r) = 4\epsilon[(\sigma/r)^{12} - c(\sigma/r)^6]$, with $c = 0.5$ (poor wetting), $c = 1$ (standard condition) and 2.0 (good wetting). While this affected the temperature increment $\Delta T$, the temperature profile around the nanoparticle still obeyed eq. (6) of the main text. Thus the particle only appears hotter or colder for different values of $c$, and the measured values of $T_{\rm k}$ and $T_{\rm HBM}$ fall onto the same curve if plotted as functions of $\Delta T$ (figure 4).

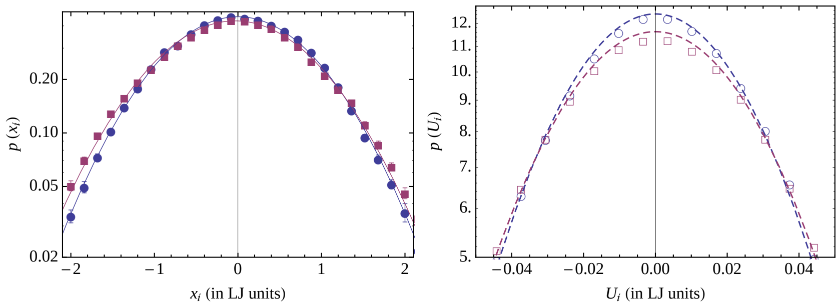


Figure 3: Distribution of the configurational and kinetic degrees of freedom for an internal/external heating mechanism. **Left**: Distribution of the coordinates of a nanoparticle that is externally heated to $T_{\rm p}$ = 1.00 ● and 1.50 ■ in a harmonic well, compared to the corresponding Boltzmann distribution for internal heating (lines). **Right**: Distribution of the center-of-mass velocities of the externally heated nanoparticle at $T_{\rm p}$ = 1.00 ○ and 1.50 □, compared to the corresponding Boltzmann distributions for internal heating (lines).

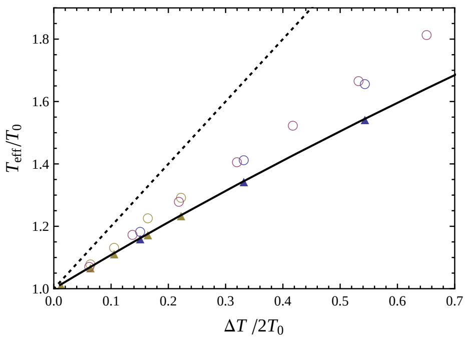


Figure 4: Dependence of the effective temperatures on the wetting parameter $c$. The open symbols (○,○,○) are the kinetic temperatures for $c$ = 0.5, 1, 2 respectively. The filled symbols ( ▲, ▲) are $T_{\rm HBM}$ for $c$ = 0.5, 2 respectively, and the solid line is the theoretically predicted $T_{\rm HBM}$ for $c$ = 1. The dashed line is the solvent temperature at the particle surface.

# References


[1] Daan Frenkel and Berend Smit. *Understanding Molecular Simulation: From Algorithms to Applications.* Academic Press, Inc., San Diego, California, USA, 2nd edition, 2002.

[2] E. H. Hauge and A. Martin-Löf. Fluctuating hydrodynamics and Brownian motion. *J. Stat. Phys.*, 7(3):259–281, March 1973.

[3] Simone Melchionna, Giovanni Ciccotti, and Brad Lee Holian. Hoover NPT dynamics for systems varying in shape and size. *Molecular Physics*, 78(3):533–544, February 1993.

[4] Daniel Rings, Romy Schachoff, Markus Selmke, Frank Cichos, and Klaus Kroy. Hot Brownian Motion. *Phys. Rev. Lett.*, 105(9):090604, Aug 2010.

[5] Daniel Rings, Markus Selmke, Frank Cichos, and Klaus Kroy. Theory of Hot Brownian Motion. *Soft Matter*, 7:3441–3452, 2011.

[6] S. Toxvaerd. Molecular dynamics at constant temperature and pressure. *Physical Review E*, 47(1):343, 1993.
